# Supplementary material for: Learning to Guide a Saturation-Based Theorem Prover
Source: arXiv:2106.03906 source file (2021-06-07)
Supplement: Supplementary file 1 [file appendix.tex]

\appendix
\section{Appendix}
\label{sec:appendix}

\subsection{Hyperparameter Tuning and Experimental Setup}
\label{sec:hyperparams}
We  used  gradient-boosted tree  search from
scikit-optimize\footnote{\url{https://scikit-optimize.github.io/}} to find effective hyper-parameters using 10\% of the Mizar dataset. This returned the hyperparameter values in Table~\ref{tab:hyperparameters}. The maximum time limit for solving a problem was 100 seconds. Hyper-parameter tuning experiments were conducted over a cluster of 19 CPU (56 x 2.0 GHz cores \& 247 GB RAM) and 10 GPU machines (2 x P100 GPU, 16 x 2.0 GHz CPU cores, \& 120 GB RAM) over 4 to 5 days.% (for hyper-parameter tuning, we added 5 CPU and 2 GPU machines).

Once the best hyperparameters were found, we ran TRAIL and its competitors (see Section 4.1 and Appendix~\ref{subsec:plcop}) on a CPU machine with 56 x 2.0 GHz cores \& 247 GB RAM. At the end of each iteration, collected training examples were shipped to a dedicated GPU server (with 2 x P100 GPUs, 16 x 2.0 GHz CPU cores, \& 120 GB RAM) which trains and updates \trail's policy network.

\begin{table}[h]
\centering
\footnotesize
\begin{tabular}{ll}
\toprule
Parameter                  & Value \\
\midrule
Chains Patterns            & 500 \\
Sub-walks                  & 2000 \\
$k$ layers                 & 2     \\
units per layer            & 161   \\
dropout                    & 0.57  \\
$\lambda$ (reg.)           & 0.004 \\
$2d$ (sparse vector size)  & 645   \\
$\tau$ (temp.)              & 1.13 \\
$\tau_0$ (temp. threshold)             & 11  \\
embedding layers           & 4  \\
dense embedding size        & 800  \\
% $\rho$ (expert decay)      & 0.75    \\
reward normalization       &  (i) normalized by difficulty\\

\bottomrule
\end{tabular}
\caption{Hyperparameter values} 
\label{tab:hyperparameters}
\end{table}

\begin{table*}[h!]
\centering
\footnotesize
\begin{tabular}{lcccccccccc}
\toprule
         & 1 & 2 & 3 & 4 & 5 & 6 & 7 & 8 & 9 & 10 \\
         \midrule
M2k &   1042	& 1266 &	1428 &	1490 &	1507 &	1527 &	1533 &	1549 &	1552 &	\bf 1561 \\
MPTP2078      & 363	& 552 &	680	& 730 &	806 &	844	& 858 &	878	& 877 &	\bf 910    \\
\bottomrule
\end{tabular}
\caption{\trail's performance across iterations}
\label{tab:trail_iter}
\end{table*}

\subsection{Underlying Reasoner}
\label{sec:underlying_reasoner}
The current implementation of \trail uses Beagle~\cite{Beagle2015} as its underlying inference execution system. This is purely an implementation choice, made primarily due to Beagle's easily modifiable open source code and friendly license. 
The purpose of Beagle in \trail is to execute the actions selected by the \trail learning agent; i.e., Beagle’s proof guidance was completely disabled when embedded as a component in \trail and whenever Beagle reaches a decision point at the level of clause selection, it delegates the decision to \trail's policy to decide the next action to pick. 
%{\color{blue} 
When \trail passes an inference action to Beagle to execute, it does not specify any additional restrictions, thus ordering constraints and literal selection specified for Beagle's default settings are used by Beagle when it executes the action. Redundancy elimination is also allowed (e.g., proper subsumption deletion), with the exception of all backward simplification techniques.
%}

Using an off-the-shelf reasoner (like Beagle) as a reasoning shell is to ensure that the set of inference rules available to \trail are both sound and complete, and that all proofs generated can be trusted. % \trail only assumes its underlying reasoner to be saturation-based and is otherwise not reasoner-dependent, i.e., and any reasoner that can apply FOL inference rules can serve the same role as Beagle in \trail. 
Beagle only executes the actions selected by \trail and can thus be replaced by any saturation-based reasoner capable of applying FOL inference rules.

\begin{figure}[h]
\begin{center}
\includegraphics[width=1.0\columnwidth]{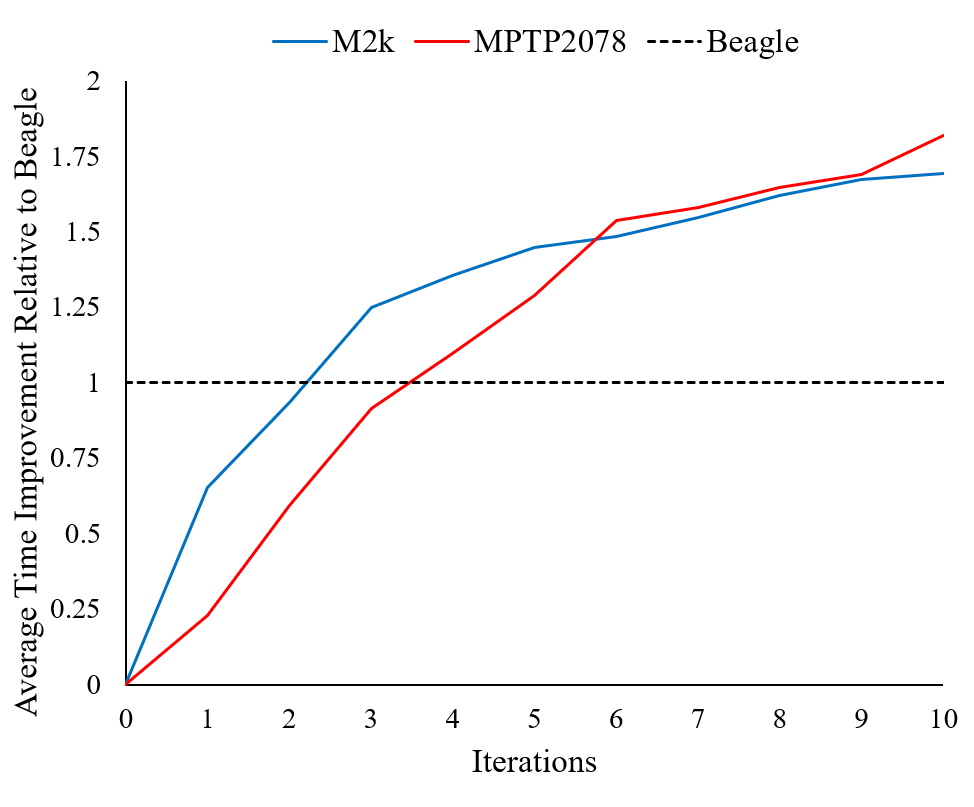}
\vspace{-0.2in}
\caption{\trail's average proof time improvement relative to Beagle (i.e., Beagle's average time to find a proof divided by \trail's average time to find a proof)}
\label{fig:proof_time}
\end{center}
\end{figure}

\subsection{\trail's Learning}
Table \ref{tab:trail_iter} shows the performance of {\trail} across iterations. Compared to the first iteration, \trail managed to solved 547 more problems on MPTP2078 and 519 more problems on M2k. This indicates that \trail is learning rather quickly, beating rlCop and plCop on both datasets by the fifth iteration of learning. Interestingly, \trail's performance monotonically increases over the iterations, which indicates that it is not overfitting to a particular subset of the problems within either dataset.

We also show in Figure \ref{fig:proof_time} the speed at which \trail finds a proof as compared to Beagle. As can be seen in the figure, \trail surpasses Beagle's speed rather quickly (at the second iteration for M2k and the fourth iteration for MPTP). 
One possibility for this is that \trail is initially solving an easier subset of problems, as evidenced by the fact that at both of those iterations, \trail is actually solving fewer problems than Beagle (see Table \ref{tab:trail_iter}). However, by the time \trail reaches iteration 8 on M2k, it solves more problems than Beagle with a 1.6x improvement in terms of time. Similarly on MPTP2078, \trail iteration 5 managed to solved more than 160 problems than Beagle in 1.29x better time. 
% This is interesting, as \trail actually solves fewer problems than Beagle (see Table \ref{tab:trail_iter}) at both of those iterations (in fact, \trail does not surpass Beagle in terms of the number of solved problems on M2k until iteration 8).

\begin{table}
\centering
\footnotesize
\resizebox{1\columnwidth}{!}{
\begin{tabular}{l l l l l l}
\toprule
 & & M2k & Stat. Sig. & MPTP2078 & Stat. Sig. \\
\toprule
\multirow{3}{*} {\setstackgap{S}{4.05ex}\Centerstack[l]{Traditional}}& E & \bf 1922 & \checkmark  (\footnotesize{$z$=-16.9})& \bf 998 & \checkmark (\footnotesize{$z$=-2.7)})\\
% The value of z is -16.9011. The value of p is < .00001. The result is significant at p < .05.
% The value of z is -2.7393. The value of p is .00614. The result is significant at p < .05.
&Beagle & 1543 & & 742 & \checkmark (\footnotesize{$z$=5.3})\\
% The value of z is 0.6803. The value of p is .4965. The result is not significant at p < .05.
% The value of z is 5.3251. The value of p is < .00001. The result is significant at p < .05.
& mlCop & 1034 & \checkmark (\footnotesize{$z$=17.4}) & 502 & \checkmark (\footnotesize{$z$=13.4})\\
% The value of z is 17.4235. The value of p is < .00001. The result is significant at p < .05.
% The value of z is 13.3625. The value of p is < .00001. The result is significant at p < .05.
\midrule
\multirow{3}{*} {\setstackgap{S}{4.05ex}\Centerstack[l]{RL-Based}}& rlCop &  1235 & \checkmark (\footnotesize{$z$=11.2}) & 733 & \checkmark (\footnotesize{$z$=5.6}) \\
% The value of z is 11.2114. The value of p is < .00001. The result is significant at p < .05.
% The value of z is 5.6156. The value of p is < .00001. The result is significant at p < .05.
& plCop & 1359 & \checkmark (\footnotesize{$z$=7.2}) & 782 & \checkmark  (\footnotesize{$z$=4.0})\\   
% The value of z is 7.1748. The value of p is < .00001. The result is significant at p < .05.
% The value of z is 4.0414. The value of p is < .00001. The result is significant at p < .05.
&\trail  & \bf{1561} & & \bf{910} & \\
\bottomrule
\end{tabular}
}
\caption{Number of problems solved in M2k and MPTP2078, best two approaches in \textbf{bold}. Statistically significant differences ($p$ < .05) {\emph{relative to \trail}} are marked with \checkmark.
}
\label{tab:m2k_2078_stat}
\end{table}

\subsection{Statistical Significance Tests}
Table \ref{tab:m2k_2078_stat} shows the performance of \trail compared to learning and traditional theorem provers. This table repeats the results reported in Table 1 in Section 4.1 with statistical significance tests ($p < 0.05$) relative to \trail. For example, state-of-the-art traditional theorem prover E outperforms all other approaches including \trail. E outperforms \trail in a statistically significant way with $z = -16.9$ on M2k and $z = -2.7$ on MPTPT2078 dataset. On the other hand, \trail outperforms Beagle in a non-significant way on M2k ($z = 0.6$) and in a significant way on MPTP2078 ($z = 5.3$). Furthermore, all \trail's improvements over mlCop, rlCop and plCop are statistically significant.

\subsection{rlCop and plCop Experiments}
\label{subsec:plcop}

% plcop with paramodulation 		--> M2k: 1301, 2078b: 773
% plcop without paramodulation --> M2k: 1222, 2078b: 707
% rlcop with paramodulation  	 --> M2k: 1238, 2078b: 563
% rlcop without paramodulation 	 --> M2k: 1148, 2078b: 543

\begin{table}
\centering
\footnotesize
\begin{tabular}{lcc}
\toprule
      & M2k & MPTP2078 \\
\midrule
TRAIL &   \bf 1,561  &    \bf 910     \\
rlCop (w/o paramodulation) &  1,148   &  543        \\
rlCop (w/ paramodulation) & 1,238 & 563 \\
plCop (w/o paramodulation) & 1,222  & 707 \\
plCop (w/ paramodulation)&   1,301  &    773\\     
\bottomrule
\end{tabular}
\caption{plCop and rlCop performance using same hardware and time limit (100 seconds) as \trail }
\label{tab:rlcop_plcop}
\end{table}

As mentioned in Section 4.1, the numbers reported in Table 1 for plCop and rlCop are taken from their papers \cite{KalUMO-NeurIPS18-atp-rl,zombori2020prolog}. We also replicated their performance under our exact hardware and time constraints. In particular, we used the authors' source code available at \url{https://github.com/zsoltzombori/plcop} which contains the implementation of both rlCop and plCop.  
We used the same default parameters from plCop's configuration files. We noticed, however, that they have two prominent configurations for each dataset (with and without paramodulation) and as a result we decided to report both configurations on each dataset. Table~\ref{tab:rlcop_plcop} shows the performance of \trail, plCop and rlCop on the same hardware with 100 seconds time limit. plCop performance is very close to what we have in Table~1 in Section 4.1 while rlCop numbers are lower. 
To avoid any confusion, we decided to use the best performance for both rlCop and plCop in Table 1 in Section 4.1 which is what the authors reported in their paper. This experiment is to show that the hardware used and the time limits are comparable and hence fair comparison can be made.
